# Supplementary material for: Exploiting Social Tie Structure for Cooperative Wireless Networking: A Social Group Utility Maximization Framework
Source: arXiv:1605.00091 source file (2016-04-30)
Supplement: Supplementary file 1 [file Appendix.tex]

\appendix
\subsection{Proof of Theorem \ref{thm:The-social-physical-game}}\label{proof1}
Suppose that a user $k$ changes its channel $a_{k}$ to
$a_{k}^{'}$ such that the channel selection profile changes from
$\boldsymbol{a}$ to $\boldsymbol{a}^{'}$. We have that
\begin{align}
\Phi(\boldsymbol{a}^{'})-\Phi(\boldsymbol{a}) = \Phi_{1}(\boldsymbol{a}^{'})-\Phi_{1}(\boldsymbol{a})+\Phi_{2}(\boldsymbol{a}^{'})-\Phi_{2}(\boldsymbol{a}).\label{eq:PP0}
\end{align}

For the part $\Phi_{1}$, we have that
\begin{align}
   & \Phi_{1}(\boldsymbol{a}^{'})-\Phi_{1}(\boldsymbol{a})\nonumber \\
  = & -\frac{1}{2}\sum_{m\in\mathcal{N}_{k}^{p}}P_{m}d_{mk}^{-\alpha}I_{\{a_{k}^{'}=a_{m}\}}-\frac{1}{2}\sum_{n\neq k}\sum_{k\in\mathcal{N}_{n}^{p}}P_{k}d_{kn}^{-\alpha}I_{\{a_{n}=a_{k}^{'}\}}\nonumber \\
  & -\omega_{a_{k}^{'}}^{k} +\frac{1}{2}\sum_{m\in\mathcal{N}_{k}^{p}}P_{m}d_{mk}^{-\alpha}I_{\{a_{k}=a_{m}\}}\nonumber \\
  & +\frac{1}{2}\sum_{n\neq k}\sum_{k\in\mathcal{N}_{n}^{p}}P_{k}d_{kn}^{-\alpha}I_{\{a_{n}=a_{k}\}}+\omega_{a_{k}}^{k}.\label{eq:PP1}
\end{align}
Since users access the spectrum with the same power level and the interference relationship and distance measurement are symmetry, we know
that
\begin{align}
\sum_{n\neq k}\sum_{k\in\mathcal{N}_{n}^{p}}P_{k}d_{kn}^{-\alpha}  = \sum_{n\in\mathcal{N}_{k}^{p}}P_{k}d_{kn}^{-\alpha} = \sum_{n\in\mathcal{N}_{k}^{p}}P_{n}d_{nk}^{-\alpha}.\label{eq:PP2}
\end{align}
Combining (\ref{eq:PP1}) and (\ref{eq:PP2}), we
have that
\begin{align}
   & \Phi_{1}(\boldsymbol{a}^{'})-\Phi_{1}(\boldsymbol{a})\nonumber \\
  = & -\frac{1}{2}\sum_{m\in\mathcal{N}_{k}^{p}}P_{m}d_{mk}^{-\alpha}I_{\{a_{k}^{'}=a_{m}\}}-\frac{1}{2}\sum_{n\in\mathcal{N}_{k}^{p}}P_{n}d_{nk}^{-\alpha}I_{\{a_{n}=a_{k}^{'}\}}-\omega_{a_{k}^{'}}^{k}\nonumber \\
   & +\frac{1}{2}\sum_{m\in\mathcal{N}_{k}^{p}}P_{m}d_{mk}^{-\alpha}I_{\{a_{k}=a_{m}\}}+\frac{1}{2}\sum_{n\in\mathcal{N}_{k}^{p}}P_{n}d_{nk}^{-\alpha}I_{\{a_{n}=a_{k}\}}+\omega_{a_{k}}^{k}\nonumber \\
  = & -\sum_{m\in\mathcal{N}_{k}^{p}}P_{m}d_{mk}^{-\alpha}I_{\{a_{k}^{'}=a_{m}\}}-\omega_{a_{k}^{'}}^{k}\nonumber \\
   & +\sum_{m\in\mathcal{N}_{k}^{p}}P_{m}d_{mk}^{-\alpha}I_{\{a_{k}=a_{m}\}}+\omega_{a_{k}}^{k}\nonumber \\
  = & -\gamma_{k}(\boldsymbol{a}^{'})+\gamma_{k}(\boldsymbol{a})= U_{k}(\boldsymbol{a}^{'})-U_{k}(\boldsymbol{a}).\label{eq:PP4}
\end{align}

Similarly, for the part $\Phi_{2}$, we have that
\begin{align}
  & \Phi_{2}(\boldsymbol{a}^{'})-\Phi_{2}(\boldsymbol{a})\nonumber \\
  %= & -  \sum_{n\in\mathcal{N}_{k}^{sp}}w_{kn}P_{k}d_{kn}^{-\alpha}I_{\{a_{n}=a_{k}^{'}\}}+\sum_{n\in\mathcal{N}_{k}^{sp}}w_{kn}P_{k}d_{kn}^{-\alpha}I_{\{a_{n}=a_{k}\}}\nonumber \\
  = & \sum_{n\in\mathcal{N}_{k}^{sp}}w_{kn}\left(-P_{k}d_{kn}^{-\alpha}I_{\{a_{n}=a_{k}^{'}\}}+P_{k}d_{kn}^{-\alpha}I_{\{a_{n}=a_{k}\}}\right)\nonumber \\
  = & \sum_{n\in\mathcal{N}_{k}^{sp}}w_{kn}\times \nonumber \\
  & \left(-P_{k}d_{kn}^{-\alpha}I_{\{a_{n}=a_{k}^{'}\}}-\sum_{m\neq k}\sum_{m\in\mathcal{N}_{n}^{p}}P_{m}d_{mn}^{-\alpha}I_{\{a_{n}=a_{m}\}}-\omega_{a_{n}}^{k}\right.\nonumber \\
   & \left.+P_{k}d_{kn}^{-\alpha}I_{\{a_{n}=a_{k}\}}+\sum_{m\neq k}\sum_{m\in\mathcal{N}_{n}^{p}}P_{m}d_{mn}^{-\alpha}I_{\{a_{n}=a_{m}\}}+\omega_{a_{n}}^{k}\right)\nonumber \\
  = & \sum_{n\in\mathcal{N}_{k}^{sp}}w_{kn}\left(-\gamma_{n}(\boldsymbol{a}^{'})+\gamma_{n}(\boldsymbol{a})\right)\nonumber \\
  = & \sum_{n\in\mathcal{N}_{k}^{sp}}w_{kn}\left(U_{n}(\boldsymbol{a}^{'})-U_{n}(\boldsymbol{a})\right).\label{eq:PP8}
\end{align}

Finally, substituting (\ref{eq:PP4}) and (\ref{eq:PP8}) into (\ref{eq:PP0}),
we obtain that
\begin{align}
   & \Phi(\boldsymbol{a}^{'})-\Phi(\boldsymbol{a})\nonumber \\
  = & U_{k}(\boldsymbol{a}^{'})-U_{k}(\boldsymbol{a})+\sum_{n\in\mathcal{N}_{k}^{sp}}w_{kn}\left(U_{n}(\boldsymbol{a}^{'})-U_{n}(\boldsymbol{a})\right).\label{eq:PP9}
\end{align}
Since user $k$ can not generate interference to any user $n\in\mathcal{N}_{k}^{s}\backslash\mathcal{N}_{k}^{sp}$,
we have that
\[
U_{n}(\boldsymbol{a}^{'})=U_{n}(\boldsymbol{a}),\forall n\in\mathcal{N}_{k}^{s}\backslash\mathcal{N}_{k}^{sp}.
\]
This implies that
\begin{align*}
   & \Phi(\boldsymbol{a}^{'})-\Phi(\boldsymbol{a})\\
  = & U_{k}(\boldsymbol{a}^{'})-U_{k}(\boldsymbol{a})+\sum_{n\in\mathcal{N}_{k}^{sp}}w_{kn}\left(U_{n}(\boldsymbol{a}^{'})-U_{n}(\boldsymbol{a})\right)\\
 & +\sum_{n\in\mathcal{N}_{k}^{s}\backslash\mathcal{N}_{k}^{sp}}w_{kn}\left(U_{n}(\boldsymbol{a}^{'})-U_{n}(\boldsymbol{a})\right)\\
  = & U_{k}(\boldsymbol{a}^{'})-U_{k}(\boldsymbol{a})+\sum_{n\in\mathcal{N}_{k}^{s}}w_{kn}\left(U_{n}(\boldsymbol{a}^{'})-U_{n}(\boldsymbol{a})\right),
\end{align*}
which completes the proof. \qed

\subsection{Proof of Theorem \ref{thm:The-distributed-D2D}}\label{proof2}
As mentioned, the system state of the spectrum access Markov chain
is defined as the channel selection profile $\boldsymbol{a}\in\Theta$
of all users. Since it is possible to get from any state to any
other state within finite steps of transition, the spectrum access
Markov chain is hence irreducible and has a stationary distribution.

We then show that the Markov chain is time reversible by showing that
the distribution in (\ref{eq:qq1}) satisfies the following detailed
balance equations:
\begin{equation}
q_{\boldsymbol{a}}^{*}q_{\boldsymbol{a},\boldsymbol{a}^{'}}=q_{\boldsymbol{a}^{'}}^{*}q_{\boldsymbol{a}^{'},\boldsymbol{a}},\forall\boldsymbol{a},\boldsymbol{a}^{'}\in\Theta.\label{eq:phh7}
\end{equation}
To see this, we consider the following two cases:

1) If $\boldsymbol{a}^{'}\notin\Delta_{\boldsymbol{a}}$, we have
$q_{\boldsymbol{a},\boldsymbol{a}^{'}}=q_{\boldsymbol{a}^{'},\boldsymbol{a}}=0$
and the equation (\ref{eq:phh7}) holds.

2) If $\boldsymbol{a}^{'}\in\Delta_{\boldsymbol{a}}$, according to
(\ref{eq:qq1}) and (\ref{eq:PPP4}), we have
\begin{eqnarray*}
 &  & q_{\boldsymbol{a}}^{*}q_{\boldsymbol{a},\boldsymbol{a}^{'}}\\
 & = & \frac{\tau_{n}}{|\mathcal{M}_{n}|}\frac{\exp(\theta\Phi(\boldsymbol{a}))}{\sum_{\hat{\boldsymbol{a}}\in\Theta}\exp(\theta\Phi(\hat{\boldsymbol{a}}))}\\
 &  & \times\frac{\exp\left(\theta S_{n}(a_{n}^{'},a_{-n})\right)}{\max\{\exp\left(\theta S_{n}(a_{n}^{'},a_{-n})\right), \exp\left(\theta S_{n}(a_{n},a_{-n})\right)\}}\\
 & = & \frac{\tau_{n}}{|\mathcal{M}_{n}|}\frac{\exp\left(\theta\left(\Phi(\boldsymbol{a})+ S_{n}(a_{n}^{'},a_{-n})\right)\right)}{\sum_{\hat{\boldsymbol{a}}\in\Theta}\exp(\theta\Phi(\hat{\boldsymbol{a}}))}\\
 &  & \times\frac{1}{\max\{\exp\left(\theta S_{n}(a_{n}^{'},a_{-n})\right), \exp\left(\theta S_{n}(a_{n},a_{-n})\right)\}},
\end{eqnarray*}
and similarly,
\begin{eqnarray*}
 &  & q_{\boldsymbol{a}^{'}}^{*}q_{\boldsymbol{a}^{'},\boldsymbol{a}}\\
 & = & \frac{\tau_{n}}{|\mathcal{M}_{n}|}\frac{\exp\left(\theta\left(\Phi(\boldsymbol{a}^{'})+ S_{n}(a_{n},a_{-n})\right)\right)}{\sum_{\hat{\boldsymbol{a}}\in\Theta}\exp(\theta\Phi(\hat{\boldsymbol{a}}))}\\
 &  & \times\frac{1}{\max\{\exp\left(\theta S_{n}(a_{n}^{'},a_{-n})\right), \exp\left(\theta S_{n}(a_{n},a_{-n})\right)\}}.
\end{eqnarray*}
Thus, according to (\ref{eq:Potential}), we must have
\begin{eqnarray*}
 &  & q_{\boldsymbol{a}}^{*}q_{\boldsymbol{a},\boldsymbol{a}^{'}}=q_{\boldsymbol{a}^{'}}^{*}q_{\boldsymbol{a}^{'},\boldsymbol{a}}.
\end{eqnarray*}
The spectrum access Markov chain is hence time-reversible and has
the unique stationary distribution as given in (\ref{eq:qq1}). \qed

\subsection{Proof of Theorem~\ref{thm:mixing}}\label{proof33}
\rev{
(a) For the first part, we prove the result based on the spectral analysis method for mixing
time \cite{levin2009markov,chen2010markov}. First, the the spectrum access Markov chain
is a continuous-time Markov chain with the stationary distribution
given as
\[
q_{\boldsymbol{a}}^{*}=\frac{\exp(\theta\Phi(\boldsymbol{a}))}{\sum_{\hat{\boldsymbol{a}}\in\Omega}\exp(\theta\Phi(\hat{\boldsymbol{a}}))},\forall\boldsymbol{a}\in\Omega.
\]
Since $\sum_{\hat{\boldsymbol{a}}\in\Omega}\exp(\theta\Phi(\hat{\boldsymbol{a}}))\leq|\Omega|\exp(\theta\Phi_{\max})$
and $|\Omega|=\prod_{n=1}^{N}|\mathcal{M}_{n}|$, then the minimum
probability in the stationary distribution is
\begin{eqnarray}
q_{\min}^{*} & \triangleq & \min_{\boldsymbol{a}\in\Omega}q_{\boldsymbol{a}}^{*} \geq \frac{\exp(\theta\Phi_{\min})}{|\Omega|\exp(\theta\Phi_{\max})}\nonumber \\
 & \geq & \frac{\exp(-\theta(\Phi_{\max}-\Phi_{\min}))}{M_{\max}^{N}}.\label{eq:mt1}
\end{eqnarray}

Using the spectral analysis method \cite{levin2009markov}, we carry out
the uniformization over the continuous-time spectrum access Markov
chain. We denote $Q\triangleq\{q_{\boldsymbol{a},\boldsymbol{a}^{'}}\}$
as the transition rate matrix of the spectrum access Markov chain
and construct a discrete-time Markov chain $D(t)$ with the transition
matrix $P\triangleq\{p_{\boldsymbol{a},\boldsymbol{a}^{'}}\}=I+\frac{Q}{\xi}$,
where $\xi$ is the uniform rate parameter satisfying $\xi\geq\max_{\boldsymbol{a}\in\Omega}\sum_{\boldsymbol{a}^{'}\neq\boldsymbol{a}}q_{\boldsymbol{a},\boldsymbol{a}^{'}}$.
Since $q_{\boldsymbol{a},\boldsymbol{a}^{'}}=\frac{\tau_{n}}{|\mathcal{M}_{n}|}\frac{\exp(\theta S_{n}(\boldsymbol{a}))}{\max\{\exp(\theta S_{n}(\boldsymbol{a})),\exp(\theta S_{n}(\boldsymbol{a}^{'}))\}},$
it follows that
\begin{equation}
\frac{\tau_{\min}}{M_{\max}}\exp(-\theta\varDelta)\leq q_{\boldsymbol{a},\boldsymbol{a}^{'}}\leq\frac{\tau_{\max}}{M_{\min}},\forall\boldsymbol{a},\boldsymbol{a}^{'}\in\Omega,
\end{equation}
where $\varDelta=\max_{n\in\mathcal{N},\boldsymbol{a},\boldsymbol{a}^{'}\in\Omega}|S_{n}(\boldsymbol{a})-S_{n}(\boldsymbol{a}^{'})|$. Hence, we have
\begin{equation}
\frac{\tau_{\min}}{M_{\max}}\exp(-\theta(\Phi_{\max}-\Phi_{\min}))\leq q_{\boldsymbol{a},\boldsymbol{a}^{'}}\leq\frac{\tau_{\max}}{M_{\min}},\forall\boldsymbol{a},\boldsymbol{a}^{'}\in\Omega. \label{eq:mt2}
\end{equation}

Due to the fact that from a state $\boldsymbol{a}$, the Markov chain
can transit to at most $M_{\max}N$ other states, we now have that
$\max_{\boldsymbol{a}\in\Omega}\sum_{\boldsymbol{a}^{'}\neq\boldsymbol{a}}q_{\boldsymbol{a},\boldsymbol{a}^{'}}\leq\frac{M_{\max}\tau_{\max}}{M_{\min}}N$
and we can hence set the uniform rate parameter $\xi=\frac{M_{\max}\tau_{\max}}{M_{\min}}N$.

Then, based on the spectral gap inequality \cite{levin2009markov}, it follows that
\begin{eqnarray*}
\max_{\boldsymbol{a}_{0}\in\Omega}||\boldsymbol{q}_{t}(\boldsymbol{a}_{0})-\boldsymbol{q}^{*}||_{TV} & \leq & \frac{\exp(-\xi(1-\lambda_{2})t)}{2\sqrt{q_{\min}^{*}}},
\end{eqnarray*}
where $\lambda_{2}$ is the second largest eigenvalue of transition
matrix for the discrete-time Markov chain $D(t)$ by uniformization.
Therefore, the mixing time $T_{\epsilon}$ satisfies that
\begin{equation}
T_{\epsilon}\leq\frac{\ln\frac{1}{2\epsilon}+\frac{1}{2}\ln\frac{1}{q_{\min}^{*}}}{\xi(1-\lambda_{2})}.\label{eq:tm3}
\end{equation}
Furthermore, applying Cheeger's Inequality \cite{levin2009markov}, we have that
\[
1-\lambda_{2}\geq\frac{\varphi^{2}}{2},
\]
 where
\begin{eqnarray}
\varphi & \triangleq & \min_{\boldsymbol{a}^{'}\neq\boldsymbol{a},q_{\boldsymbol{a},\boldsymbol{a}^{'}}>0}q_{\boldsymbol{a}}^{*}\frac{q_{\boldsymbol{a},\boldsymbol{a}^{'}}}{\xi},\label{eq:tm4}
\end{eqnarray}
implying that
\begin{eqnarray}
 &  & \varphi\geq\frac{q_{\min}^{*}\frac{\tau_{\min}}{M_{\max}}\exp(-\theta\varDelta)}{\xi}.\label{eq:tm5}
\end{eqnarray}

Combining (\ref{eq:mt1}), (\ref{eq:mt2}), (\ref{eq:tm3}), (\ref{eq:tm4}),
and (\ref{eq:tm5}), we finally conclude  that
\begin{align*}
T_{\epsilon}  \leq & \frac{2\ln\frac{1}{2\epsilon}+\ln\frac{1}{q_{\min}^{*}}}{\xi\varphi^{2}} \leq  \xi\exp(2\theta\varDelta)\frac{2\ln\frac{1}{2\epsilon}+\ln\frac{1}{q_{\min}^{*}}}{\left(q_{\min}^{*}\frac{\tau_{\min}}{M_{\max}}\right)^{2}}\\
  \leq & \frac{NM_{\max}^{2N+3}\tau_{\max}}{M_{\min}\tau_{\min}^{2}}\exp\left(4\theta(\Phi_{\max}-\Phi_{\min})\right)\\
   & \times\left[2\ln\frac{1}{2\epsilon}+N\ln M_{\max}+\theta(\Phi_{\max}-\Phi_{\min})\right].
\end{align*}

(b) For the second part, we analyze the mixing time using the coupling method \cite{levin2009markov}.
The key idea is to carefully construct a discrete-time Markov chain
that satisfies the spectrum access Markov chain uniformization condition,
and then show this discrete-time Markov chain possesses the one-step
path coupling property when $\theta<\theta_{th}$. By doing so, we
can derive a tighter upper-bound of the mixing time of the spectrum
access Markov chain.

First of all, according to the result in Part (a), we can define the
discrete-time Markov chain $D(t)$ such that at each step, a user
$n$ is selected purely randomly for the channel update. Specifically,
for each time slot, we carry out the following: 1) choose a user $n\in\mathcal{N}$
with a probability $\frac{1}{N}$; 2) choose a new channel $a_{n}^{'}$
randomly with $\frac{1}{|\mathcal{M}_{n}|}$; 3) let user $n$ switch
to the new channel with a probability $\frac{M_{\min}\tau_{n}}{M_{\max}\tau_{\max}}\frac{\exp(\theta S_{n}(\boldsymbol{a}))}{\max\{\exp(\theta S_{n}(\boldsymbol{a})),\exp(\theta S_{n}(\boldsymbol{a}^{'}))\}}$.
As shown in Part (a), such discrete-time Markov chain has the transition
matrix $P\triangleq\{p_{\boldsymbol{a},\boldsymbol{a}^{'}}\}=I+\frac{Q}{\xi}$,
with $\xi$ being the uniformization parameter $\xi=\frac{M_{\max}\tau_{\max}}{M_{\min}}N$.

We then apply the coupling method to derive the mixing time of the
Markov chain $D(t)$. Here a coupling of the Markov chain $D(t)$
presents a joint stochastic process $(X_{t},Y_{t})$ on $\varOmega\times\varOmega$
such that $X_{t}$ and $Y_{t}$ are the copies of the original Markov
chain $D(t)$ with the transition matrix $P$. Let $d(X_{t},Y_{t})$
denote the Hamming distance between the system states $X_{t}$ and
$Y_{t}$, which equals the number of users with different accessed
channels between these two states. The Markov chain $D(t)$ satisfies
the one-step path coupling condition, if $E[d(X_{t+1},Y_{t+1})|X_{t},Y_{t}]\leq\eta d(X_{t},Y_{t}),$
where $\eta\in[0,1)$.

Since it is difficult to analyze the couplings for all pairs $X_{t},Y_{t}\in\Omega$,
according to the path coupling technique \cite{levin2009markov}, we can restrict
attention to the pairs in a connected subset $\varUpsilon=\{(X_{t},Y_{t})\in\varOmega\times\varOmega:d(X_{t},Y_{t})=1\}$, i.e., those pairs with one step difference. Let $a_{i}(Z)$ denote user $i$'s channel selection at a state $Z$. Without loss of generality, for a pair $(X_{t},Y_{t})\in\varUpsilon$,
we assume only user $1$ chooses different channels, and the other
users choose the same channels at the states $X_{t},Y_{t}$, respectively.
That is, $a_{1}(X_{t})\neq a_{1}(Y_{t})$ and $a_{i}(X_{t})=a_{i}(Y_{t})$
for any $i\neq1$.

Now at the time slot $t+1$, a user $n$ is randomly selected to update
channel, resulting in the pair transition from $(X_{t},Y_{t})$ to
($X_{t+1},Y_{t+1}$). We denote $p_{k,n}=Pr\{a_{n}(X_{t+1})=k\}$
and $q_{k,n}=Pr\{a_{n}(Y_{t+1})=k\}$. We consider the following two
cases:

(1) When $n\neq1$, we have $a_{i}(X_{t})=a_{i}(Y_{t})$. Without
loss of generality, we assume $a_{i}(X_{t})=a_{i}(Y_{t})=1$. In this
case, for $k\neq1,$we have

\begin{eqnarray*}
p_{k,n} & = & \frac{M_{\min}\tau_{n}}{M_{\max}\tau_{\max}}\frac{\exp(\theta S_{n}(X_{t}))}{\max\{\exp(\theta S_{n}(X_{t})),\exp(\theta S_{n}(X_{t+1}))\}}\\
 & \geq & \frac{M_{\min}\tau_{\min}}{M_{\max}\tau_{\max}}\exp(-\theta(\Phi_{\max}-\Phi_{\min})).
\end{eqnarray*}
Similarly, for $k\neq1,$ we have
\[
q_{k,n}\geq\frac{M_{\min}\tau_{\min}}{M_{\max}\tau_{\max}}\exp(-\theta(\Phi_{\max}-\Phi_{\min})).
\]
And when $k=1,$ since $X_{t}=X_{t+1}$ and $Y_{t}=Y_{t+1}$, we have
\begin{eqnarray*}
p_{1,n} & = & q_{1,n}\\
 & = & \frac{M_{\min}\tau_{n}}{M_{\max}\tau_{\max}}\geq\frac{M_{\min}\tau_{\min}}{M_{\max}\tau_{\max}}\exp(-\theta(\Phi_{\max}-\Phi_{\min})).
\end{eqnarray*}

(2) When $n=1$, we have $a_{i}(X_{t})\neq a_{i}(Y_{t})$. Without
loss of generality, we assume $a_{i}(X_{t})=1$ and $a_{i}(Y_{t})=2$.
In this case, we have
\begin{eqnarray*}
p_{1,n} & = & q_{2,n}\\
 & = & \frac{M_{\min}\tau_{n}}{M_{\max}\tau_{\max}}\geq\frac{M_{\min}\tau_{\min}}{M_{\max}\tau_{\max}}\exp(-\theta(\Phi_{\max}-\Phi_{\min})),
\end{eqnarray*}
and for $k\neq1$,
\begin{eqnarray*}
p_{k,n} & = & \frac{M_{\min}\tau_{n}}{M_{\max}\tau_{\max}}\frac{\exp(\theta S_{n}(X_{t}))}{\max\{\exp(\theta S_{n}(X_{t})),\exp(\theta S_{n}(X_{t+1}))\}}\\
 & \geq & \frac{M_{\min}\tau_{\min}}{M_{\max}\tau_{\max}}\exp(-\theta(\Phi_{\max}-\Phi_{\min})).
\end{eqnarray*}
Similarly, for $k\neq2,$ we have
\[
q_{k,n}\geq\frac{M_{\min}\tau_{\min}}{M_{\max}\tau_{\max}}\exp(-\theta(\Phi_{\max}-\Phi_{\min})).
\]

Let $r_{k,n}=\min\{p_{k,n},q_{k,n}\}$. It is known from \cite{levin2009markov,chen2010markov} that
\[
E[d(X_{t+1},Y_{t+1})|X_{t},Y_{t},n=1]=1-\sum_{k=1}^{|\mathcal{M}_{n}|}r_{k,n},
\]
\[
E[d(X_{t+1},Y_{t+1})|X_{t},Y_{t},n\neq1]=2-\sum_{k=1}^{|\mathcal{M}_{n}|}r_{k,n},
\]
which imply that
\begin{eqnarray*}
 &  & E[d(X_{t+1},Y_{t+1})|X_{t},Y_{t}]\\
 & = & \sum_{i=1}^{N}Pr\{n=i\}E[d(X_{t+1},Y_{t+1})|X_{t},Y_{t},n=i]\\
 & = & \frac{1}{N}\left(2N-1-\sum_{n=1}^{N}\sum_{k=1}^{|\mathcal{M}_{n}|}r_{k,n}\right)\\
 & \leq & \frac{1}{N}\left(2N-1-\frac{NM_{\min}^{2}\tau_{\min}}{M_{\max}\tau_{\max}}\exp(-\theta(\Phi_{\max}-\Phi_{\min}))\right).
\end{eqnarray*}
Thus, when $\theta<\theta_{th}=\frac{1}{\Phi_{\max}-\Phi_{\min}}\ln\left(\frac{NM_{\min}^{2}\tau_{\min}}{(N-1)M_{\max}\tau_{\max}}\right),$ we have $L=\frac{1}{N}\left(\frac{NM_{\min}^{2}\tau_{\min}}{M_{\max}\tau_{\max}}\exp(-\theta(\Phi_{\max}-\Phi_{\min}))+1-N\right)>0$, and
\begin{align*}
E[d(X_{t+1},Y_{t+1})|X_{t},Y_{t}]< & 1-\frac{L}{N}\\
  = & \left(1-\frac{L}{N}\right)d(X_{t},Y_{t}),
\end{align*}
which satisfies the one step path coupling condition.

Then, regarding to the mixing time bound of the original Markov chain,
we know from \cite{levin2009markov,chen2010markov} that
\begin{eqnarray*}
 &  & ||\boldsymbol{q}_{t}(\boldsymbol{a}_{0})-\boldsymbol{q}^{*}||_{TV}\\
 & \leq & N\exp\left(-\xi T_{\epsilon}\frac{L}{N}\right)\\
 & = & N\exp\left(-\frac{M_{\max}\tau_{\max}}{M_{\min}}T_{\epsilon}L\right).
\end{eqnarray*}
It follows that
\[
T_{\epsilon}\leq\ln\frac{N}{\epsilon}\frac{M_{\min}}{M_{\max}\tau_{\max}L}.
\]

\qed
}

\subsection{Proof of Theorem~\ref{thm:For-the-distributed-1}}\label{proof6666}
First of all, we must have that $\Phi^{*}\geq\Phi_{\theta}$.

According to (\ref{eq:pp4}) and (\ref{eq:pp5}), we then have that
\begin{equation}
\max_{(q_{\boldsymbol{a}}:\boldsymbol{a}\in\Omega)}\sum_{a\in\Omega}q_{a}\Phi(\boldsymbol{a})\leq\max_{(q_{\boldsymbol{a}}:\boldsymbol{a}\in\Omega)}\sum_{a\in\Omega}q_{a}\Phi(\boldsymbol{a})-\frac{1}{\theta}\sum_{a\in\Omega}q_{a}\ln q_{a},\label{eq:hhhhh1}
\end{equation}
which is due to the fact that $0\leq-\frac{1}{\theta}\sum_{a\in\Omega}q_{a}\ln q_{a}\leq\frac{1}{\theta}\ln|\Omega|$.
Since $q_{a}^{*}$ is the optimal solution to (\ref{eq:pp5}) and
$\Phi^{*}=\max_{(q_{\boldsymbol{a}}:\boldsymbol{a}\in\Omega)}\sum_{a\in\Omega}q_{a}\Phi(\boldsymbol{a})$,
according to (\ref{eq:hhhhh1}), we know that
\begin{align*}
\Phi^{*} & \leq  \sum_{a\in\Omega}q_{a}^{*}\Phi(\boldsymbol{a})-\frac{1}{\theta}\sum_{a\in\Omega}q_{a}^{*}\ln q_{a}^{*}\\
 & \leq  \sum_{a\in\Omega}q_{a}^{*}\Phi(\boldsymbol{a})+\frac{1}{\theta}\ln|\Omega| \leq  \Phi_{\theta}+\frac{1}{\theta}\ln|\Omega|,
\end{align*}
which completes the proof. \qed

\subsection{Proof of Theorem~\ref{thm:The-performance-gap1}}\label{proof3333}
Let $\hat{\boldsymbol{a}}$ as the convergent SNE by the distributed spectrum access algorithm when $\theta \rightarrow \infty$ (i.e., $\hat{\boldsymbol{a}}=\arg\max_{a\in\Omega}\Phi(\boldsymbol{a})$). According to (\ref{eq:interference1}) and (\ref{eq:potential2}),
we have that
\begin{align*}
V(\boldsymbol{a})  = & \sum_{n=1}^{N}U_{n}(\boldsymbol{a})= -\sum_{n=1}^{N}\sum_{m\in\mathcal{N}_{n}^{p}}P_{m}d_{mn}^{-\alpha}I_{\{a_{n}=a_{m}\}}-\sum_{n=1}^{N}\omega_{a_{n}}^{n}\\
 % = & -\frac{1}{2}\sum_{n=1}^{N}\sum_{m\in\mathcal{N}_{n}^{p}}P_{m}d_{mn}^{-\alpha}I_{\{a_{n}=a_{m}\}}-\sum_{n=1}^{N}\omega_{a_{n}}^{n}\\
%   & -\frac{1}{2}\sum_{n=1}^{N}\sum_{m\in\mathcal{N}_{n}^{sp}}w_{nm}P_{m}d_{mn}^{-\alpha}I_{\{a_{n}=a_{m}\}}\\
%   & -\frac{1}{2}\sum_{n=1}^{N}\sum_{m\in\mathcal{N}_{n}^{sp}}(1-w_{nm})P_{m}d_{mn}^{-\alpha}I_{\{a_{n}=a_{m}\}}\\
%   & -\frac{1}{2}\sum_{n=1}^{N}\sum_{m\in\mathcal{N}_{n}^{p}\backslash\mathcal{N}_{n}^{sp}}P_{m}d_{mn}^{-\alpha}I_{\{a_{n}=a_{m}\}}\\
  = & \Phi(\boldsymbol{a})-\frac{1}{2}\sum_{n=1}^{N}\sum_{m\in\mathcal{N}_{n}^{sp}}(1-w_{nm})P_{m}d_{mn}^{-\alpha}I_{\{a_{n}=a_{m}\}}\\
   & -\frac{1}{2}\sum_{n=1}^{N}\sum_{m\in\mathcal{N}_{n}^{p}\backslash\mathcal{N}_{n}^{sp}}P_{m}d_{mn}^{-\alpha}I_{\{a_{n}=a_{m}\}}.
\end{align*}
We then have that
\begin{align}
\rho  = & V(\overline{\boldsymbol{a}})-V(\hat{\boldsymbol{a}})= \Phi(\overline{\boldsymbol{a}})-\Phi(\hat{\boldsymbol{a}})\nonumber \\
   & -\frac{1}{2}\sum_{n=1}^{N}\sum_{m\in\mathcal{N}_{n}^{sp}}(1-w_{nm})P_{m}d_{mn}^{-\alpha}\left(I_{\{\overline{a}_{n}=\overline{a}_{m}\}}-I_{\{\hat{a}_{n}=\hat{a}_{m}\}}\right)\nonumber \\
   & -\frac{1}{2}\sum_{n=1}^{N}\sum_{m\in\mathcal{N}_{n}^{p}\backslash\mathcal{N}_{n}^{sp}}P_{m}d_{mn}^{-\alpha}\left(I_{\{\overline{a}_{n}=\overline{a}_{m}\}}-I_{\{\hat{a}_{n}=\hat{a}_{m}\}}\right).\label{eq:hhhes}
\end{align}
Since $\Phi(\hat{\boldsymbol{a}})=\max_{a\in\Omega}\Phi(\boldsymbol{a})\geq\Phi(\overline{\boldsymbol{a}})$
and $V(\overline{\boldsymbol{a}})=\max_{a\in\Omega}V(\boldsymbol{a})\geq V(\hat{\boldsymbol{a}})$,
we know from (\ref{eq:hhhes}) that
\begin{align*}
\rho \leq & \frac{1}{2}\sum_{n=1}^{N}\sum_{m\in\mathcal{N}_{n}^{sp}}(1-w_{nm})P_{m}d_{mn}^{-\alpha}\left(I_{\{\hat{a}_{n}=\hat{a}_{m}\}}-I_{\{\overline{a}_{n}=\overline{a}_{m}\}}\right)\\
   & +\frac{1}{2}\sum_{n=1}^{N}\sum_{m\in\mathcal{N}_{n}^{p}\backslash\mathcal{N}_{n}^{sp}}P_{m}d_{mn}^{-\alpha}\left(I_{\{\hat{a}_{n}=\hat{a}_{m}\}}-I_{\{\overline{a}_{n}=\overline{a}_{m}\}}\right)\\
  \leq & \frac{1}{2}\sum_{n=1}^{N}\sum_{m\in\mathcal{N}_{n}^{sp}}(1-w_{nm})P_{m}d_{mn}^{-\alpha}+\frac{1}{2}\sum_{n=1}^{N}\sum_{m\in\mathcal{N}_{n}^{p}\backslash\mathcal{N}_{n}^{sp}}P_{m}d_{mn}^{-\alpha}.
\end{align*}

Then we know that
\begin{eqnarray*}
\rho & = & V(\overline{\boldsymbol{a}})-V_{\theta}\\
 & = & \sum_{\theta\in\Omega}q_{\boldsymbol{a}}^{*}(V(\overline{\boldsymbol{a}})-V(\boldsymbol{a}))\\
 & \leq & \sum_{\theta\in\Omega}q_{\boldsymbol{a}}^{*}(\Phi(\overline{\boldsymbol{a}})-\Phi(\boldsymbol{a})\\
 &  & +\frac{1}{2}\sum_{n=1}^{N}\sum_{m\in\mathcal{N}_{n}^{sp}}(1-w_{nm})P_{m}d_{mn}^{-\alpha}\\
 &  & +\frac{1}{2}\sum_{n=1}^{N}\sum_{m\in\mathcal{N}_{n}^{p}\backslash\mathcal{N}_{n}^{sp}}P_{m}d_{mn}^{-\alpha}\\
 & = & \Phi(\overline{\boldsymbol{a}})-\sum_{\theta\in\Omega}q_{\boldsymbol{a}}^{*}\Phi(\boldsymbol{a})\\
 &  & +\frac{1}{2}\sum_{n=1}^{N}\sum_{m\in\mathcal{N}_{n}^{sp}}(1-w_{nm})P_{m}d_{mn}^{-\alpha}\\
 &  & +\frac{1}{2}\sum_{n=1}^{N}\sum_{m\in\mathcal{N}_{n}^{p}\backslash\mathcal{N}_{n}^{sp}}P_{m}d_{mn}^{-\alpha}\\
 & = & \Phi(\overline{\boldsymbol{a}})-\Phi_{\theta}\\
 &  & +\frac{1}{2}\sum_{n=1}^{N}\sum_{m\in\mathcal{N}_{n}^{sp}}(1-w_{nm})P_{m}d_{mn}^{-\alpha}\\
 &  & +\frac{1}{2}\sum_{n=1}^{N}\sum_{m\in\mathcal{N}_{n}^{p}\backslash\mathcal{N}_{n}^{sp}}P_{m}d_{mn}^{-\alpha}\\
 & \leq & \Phi(\overline{\boldsymbol{a}})-\Phi^{*}+\frac{1}{\theta}\sum_{n=1}^{N}|\mathcal{M}_{n}|\\
 &  & +\frac{1}{2}\sum_{n=1}^{N}\sum_{m\in\mathcal{N}_{n}^{sp}}(1-w_{nm})P_{m}d_{mn}^{-\alpha}\\
 &  & +\frac{1}{2}\sum_{n=1}^{N}\sum_{m\in\mathcal{N}_{n}^{p}\backslash\mathcal{N}_{n}^{sp}}P_{m}d_{mn}^{-\alpha}\\
 & \leq & \frac{1}{\theta}\sum_{n=1}^{N}|\mathcal{M}_{n}|\\
 &  & +\frac{1}{2}\sum_{n=1}^{N}\sum_{m\in\mathcal{N}_{n}^{sp}}(1-w_{nm})P_{m}d_{mn}^{-\alpha}\\
 &  & +\frac{1}{2}\sum_{n=1}^{N}\sum_{m\in\mathcal{N}_{n}^{p}\backslash\mathcal{N}_{n}^{sp}}P_{m}d_{mn}^{-\alpha}.
\end{eqnarray*} \qed

\subsection{Proof of Theorem~\ref{thm:2user_NE}}\label{proof3}

Since
\begin{align*}
U_1(p_1,p_2) &= \log\left(\frac{h_1p_1}{n_1 + g_{21}p_2}\right)  - c_1p_1 +\\
&\hspace{1.6cm} w_{12}\log\left(\frac{h_2p_2}{n_2 + g_{12}p_1}\right)- w_{12}c_2p_2,
\end{align*}
we have
\[\frac{\partial U_1(p_1,p_2)}{\partial p_1} = \frac{1}{p_1} - \frac{w_{12}g_{12}}{n_2 + g_{12}p_1} - c_1.\]
Since
\[\lim_{p_1\rightarrow 0} (\frac{1}{p_1} - \frac{w_{12}g_{12}}{n_2 + g_{12}p_1}) \ge \lim_{p_1\rightarrow 0} (\frac{1}{p_1} - \frac{w_{12}}{p_1}) = \infty\]
and
\[\lim_{p_1\rightarrow \infty} (\frac{1}{p_1} - \frac{w_{12}g_{12}}{n_2 + g_{12}p_1}) = 0\]
and
\begin{align*}
\frac{\partial \left(\frac{1}{p_1} - \frac{w_{12}g_{12}}{n_2 + g_{12}p_1}\right)}{\partial p_1} &= -\frac{1}{p_1^2} + \frac{w_{12}g_{12}^2}{(n_2 + g_{12}p_1)^2} \\
&\hspace{0cm}= \frac{(w_{12}-1)g_{12}^2p_1^2-2n_2g_{12}p_1-n_2^2}{p_1^2(n_2 + g_{12}p_1)^2} \\
&< 0,
\end{align*}
there exists a unique value of $p_1$ such that
\begin{align}\label{equation1}
\frac{1}{p_1} - \frac{w_{12}g_{12}}{n_2 + g_{12}p_1} - c_1 = 0,
\end{align}
which is also the value of $p^{SNE}_1$. Solving~\eqref{equation1}, we obtain the desired result. Similarly, we can obtain $p^{SNE}_2$. \qed

\subsection{Proof of Proposition \ref{lm:2user_social}}\label{proof4444}
Since
\begin{align*}
V(p_1,p_2) &= \log\left(\frac{h_1p_1}{n_1 + g_{21}p_2}\right)  - c_1p_1 \\
&\hspace{2.4cm}+ \log\left(\frac{h_2p_2}{n_2 + g_{12}p_1}\right)- c_2p_2
\end{align*}
we have
\[\frac{\partial V(p_1,p_2)}{\partial p_1} = \frac{1}{p_1} - \frac{g_{12}}{n_2 + g_{12}p_1} - c_1.\]
Using the same argument as in the proof of Theorem~\ref{thm:2user_NE}, the optimal value $p_1^{SO}$ of $p_1$ for $V(p_1,p_2)$ is the unique solution of
\[\frac{1}{p_1} - \frac{g_{12}}{n_2 + g_{12}p_1} - c_1 = 0.\]
In particular, we have $p^{SNE}_1 \ge p_1^{SO}$. Since $\frac{\partial V(p_1,p_2)}{\partial p_1} < 0$ when $p_1 \ge p_1^{SO}$, $V(p_1,p_2)$ is decreasing in $p_1$ when $p_1 \ge p_1^{SO}$. Using Lemma~\ref{lm:2user_NE}, $p^{SNE}_1$ is decreasing in $w_{12}$, and hence $V(p^{SNE}_1,p^{SNE}_2)$ is increasing in $w_{12}$ since $p^{SNE}_2$ is independent of $w_{12}$. Similarly, we can show that $V(p^{SNE}_1,p^{SNE}_2)$ is increasing in $w_{21}$. \qed

\subsection{Proof of Theorem~\ref{thm:log_utility}}\label{proof7777}
Since
\begin{align*}
S_i(p_i,p_{-i}) &= \log\left(\frac{h_ip_i}{n_i + \sum_{j\neq i}g_{ji}p_j}\right) - c_ip_i +\\
&\hspace{0.3cm} \sum_{k\neq i}w_{ik}\left(\log\left(\frac{h_kp_k}{n_k + \sum_{j\neq k}g_{jk}p_j}\right) -c_kp_k\right),
\end{align*}
we have
\[\frac{\partial S_i(p_i,p_{-i})}{\partial p_i} = \frac{1}{p_i} - \sum_{k\neq i}\frac{w_{ik}g_{ik}}{n_k + \sum_{j\neq k}g_{jk}p_j} - c_i.\]
Since each term in the above summation term is decreasing in $p_j$, $\forall j\in\mathcal{N}\setminus i$, it follows that
\[\frac{\partial^2 S_i(p_i,p_{-i})}{\partial p_i \partial p_j} > 0, \forall j\in\mathcal{N}\setminus i\]
which implies that the social group utility function $S_i(p_i,p_{-i})$ is supermodular. It follows from~\cite{Topkis98} that there exists at least one SNE.\qed

\subsection{Proof of Theorem~\ref{thm:random_NE}}\label{proof4}

Since \begin{align*}S_i(q_i,\mathbf{q}_{-i}) &= \log\left(z_iq_i\prod_{j\in\mathcal{I}^-_i}(1 - q_j)\right) -c_iq_i\\
& \hspace{-0.0cm}\sum_{j\neq i} w_{ij}\left[\log \left(z_jq_j\prod_{k\in\mathcal{I}^-_j}(1 - p_k)\right)-c_jq_j\right],
\end{align*}
by the first-order condition, it follows that
\begin{align}\label{derivative1}
\frac{\partial S_i(q_i,\mathbf{q}_{-i})}{\partial q_i} &= \frac{1}{q_i} - \sum_{j\in\mathcal{I}^+_i} \frac{w_{ij}}{1 - q_i} - c_i\nonumber\\
&=\frac{c_iq_i^2-(\sum_{j\in\mathcal{I}^+_i} w_{ij}+1+c_i)q_i+1}{q_i(1 - q_i)}=0.
\end{align}
Then, the smaller root of equation \eqref{derivative1} is
\begin{align*}
&\frac{\sum_{j\in\mathcal{I}^+_i} w_{ij}+1+c_i-\sqrt{(\sum_{j\in\mathcal{I}^+_i} w_{ij}+1+c_i)^2-4c_i}}{2c_i} \\
&\hspace{1.0cm}\le \frac{1+c_i-\sqrt{(1+c_i)^2-4c_i}}{2c_i}\le 1,
\end{align*}
where the first inequality follows from that the first-order derivative of the small root with respect to $w_{ij}$ is
\begin{align}\label{derivative2}
\frac{1}{2c_i}\left(1 - \frac{\sum_{j\in\mathcal{I}^+_i} w_{ij}+1+c_i}{\sqrt{(\sum_{j\in\mathcal{I}^+_i} w_{ij}+1+c_i)^2-4c_i}}\right)<0.
\end{align}
Further, the larger root of equation \eqref{derivative1} is
\begin{align*}
&\frac{\sum_{j\in\mathcal{I}^+_i} w_{ij}+1+c_i+\sqrt{(\sum_{j\in\mathcal{I}^+_i} w_{ij}+1+c_i)^2-4c_i}}{2c_i} \\
&\hspace{1.0cm}\ge \frac{1+c_i+\sqrt{(1+c_i)^2-4c_i}}{2c_i}\ge 1.
\end{align*}
Therefore, the access probability $q_i^{SNE}$ at the SNE is unique and is the small root of equation \eqref{derivative1}.  \qed

\subsection{Proof of Proposition \ref{lm:random_social}}\label{proof5555}
Since
\[V(q_1,\cdots,q_N) = \sum^N_{i=1} \left[\log\left(z_iq_i\prod_{j\in\mathcal{I}^-_i}(1 - q_j)\right)-c_iq_i\right],\]
by the first-order condition, we have
\begin{align}\label{derivative3}
\frac{\partial V(q_1,\cdots,q_N)}{\partial q_i} = \frac{c_iq_i^2-(|\mathcal{I}^+_i|+1+c_i)q_i+1}{q_i(1 - q_i)}=0.
\end{align}
Similar to the proof of Theorem \ref{thm:random_NE}, we obtain the optimal strategy $q_i^{SO}$ for maximizing $V(q_1,\cdots,q_N)$ as the smaller root of equation \eqref{derivative3}, which is
\[q_i^{SO} = \frac{|\mathcal{I}^+_i|+1+c_i-\sqrt{(|\mathcal{I}^+_i|+1+c_i)^2-4c_i}}{2c_i}.\]
Since the larger root of equation \eqref{derivative3} is
\begin{align*}
&\frac{|\mathcal{I}^+_i|+1+c_i+\sqrt{(|\mathcal{I}^+_i|+1+c_i)^2-4c_i}}{2c_i} \\
&\hspace{1.0cm}\ge \frac{1+c_i+\sqrt{(1+c_i)^2-4c_i}}{2c_i}\ge 1,
\end{align*}
we have $\frac{\partial V(q_1,\cdots,q_N)}{\partial q_i} < 0$ for $q_i \in [q_i^{SO},1]$, and hence $V(q_1,\cdots,q_N)$ is decreasing in $q_i$ when $q_i \in [q_i^{SO},1]$. Using Corollary~\ref{lm:random_NE}, $q_i^{SNE}$ is decreasing in $w_{ij}$, $\forall j\in\mathcal{I}^+_i, \forall i\in\mathcal{N}$, and hence $V(q_1^{SNE},\cdots,q_N^{SNE})$ is increasing in $w_{ij}$, $\forall j\in\mathcal{I}^+_i, \forall i\in\mathcal{N}$. \qed
